# Supplementary material for: Temperature-dependent spectral function of a Kondo impurity in an $s$-wave superconductor
Source: arXiv:1901.06779 source file (2019-04-11)
Supplement: Supplementary file 1 [file Supplemental.pdf]

# Supplementary Material for "Temperature-dependent spectrum function of a Kondo impurity in an $s-wave$ superconductor"

Chenrong Liu,[1,2] Yixuan Huang,[1] Yan Chen,[2,*] and C. S. Ting[1,†]

[1] *Texas Center for Superconductivity, University of Houston, Houston, Texas 77204, USA.*
[2] *Department of Physics and State Key Laboratory of Surface Physics, Fudan University, Shanghai 200433, China.*
(Dated: April 11, 2019)

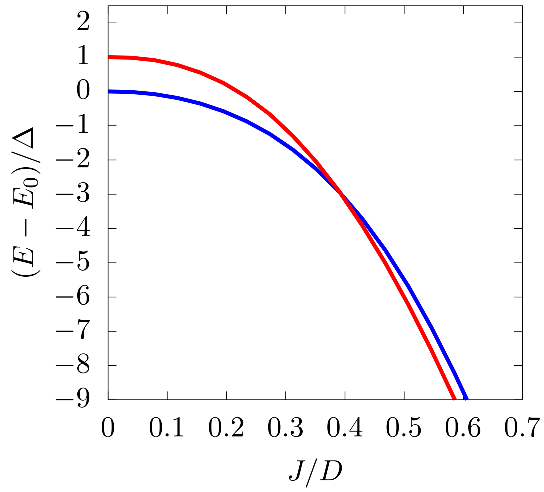


FIG. S1. (Color online) The evolutions of the impurity spin doublet-state energy (blue curve) and the impurity spin singlet-state energy (red curve) as a function of $J$ with $\Delta(0)/D = 0.01$, and $T = 0$.

## I. A. ENERGY EVOLUTION WITH KONDO COUPLING AT ZERO TEMPERATURE.

Using the NRG iteration diagonalization, it's easy to obtain the ground state energy and the first excitation energy. Here, the number of sites on the Wilson Chain is about 68, and this is enough for the high precision of diagonalization. After the last NRG iteration step, we can pick up the energy values. This is the energy level of the system. Thus, we can get the lowest energies. We noticed here that the lowest energies maybe locate in the different Hilbert space which is labeled by the good quantum number.

We first calculated the lowest two energy-level evolutions of the system by varying the Kondo coupling $J$ at $T = 0$. Near $J = 0$, the state of the impurity is spin doublet in the ground state, and the first excited state corresponds to the excitation from a Cooper pair at the impurity site, and one of the quasiparticles is then captured by the impurity spin to form a singlet state as long as the $J$ is finite. This result is shown in Fig.S1. Here we rescale the energy value by subtracting the ground state $E_0$ at $J = 0$. In the weak coupling case as $J/D < J_c/D \approx 0.39$ which corresponding to $T_k/\Delta(0) = 0.26$, the impurity spin ($S = 1/2$) could not pair with any conduction electron, and thus the ground state has doublet degeneracy. For $J > J_c$, it appears that the impurity spin can capture an electron from a Cooper pair and form a singlet ground state. This result has also been obtained by previous calculations of[1], and indicates that the impurity spin cannot be partially screened.

## II. B. THE WILSON CHAIN AND THE SPECTRUM FUNCTION.

According to the references[1,2], after applying the spherical wave representation, Eq.(1) transformed into the Wilson Chain.

$$\begin{aligned}
H =& H_k + H_\Delta + H_{imp},\\
H_k =& \frac{1+\Lambda^{-1}}{2}\sum_\sigma\sum_{n=0}^{\infty}\Lambda^{-n/2}\epsilon_n\left(f^\dagger_{n\sigma}f_{n+1\sigma}+H.c.\right),\\
H_\Delta =& -\Delta\sum_{n=0}^{\infty}\left(f^\dagger_{n\uparrow}f^\dagger_{n\downarrow}+H.c.\right),\\
H_{imp} =& \frac{J}{2}\boldsymbol{S}\cdot\sum_{\sigma\sigma'}f^\dagger_{0\sigma}\boldsymbol{\tau}_{\sigma\sigma'}f_{0\sigma'}.
\end{aligned} \tag{S1}$$

and,

$$\begin{aligned}
\epsilon_n =& \left(1-\Lambda^{-(n+1)}\right)\left(1-\Lambda^{-(2n+1)}\right)^{-1/2}\times\\
&\left(1-\Lambda^{-(2n+3)}\right)^{-1/2}
\end{aligned} \tag{S2}$$

where $\Lambda(\Lambda > 1)$ is a logarithmic discretization parameter, and we normalized the density of states of conduction electrons by $D = 1$. From Eq.S1, the first site is the impurity site while the other sites are electron sites. The Wilson Chain is a half infinity chain which means it starts from the impurity and end at the $infinity-th$ site. However, it's impossible to add infinity number sites. Due to the coefficient of the hopping term in Eq.S1 is power-law decay with the number of sites, it can be cut off at site $N_s$. $N_s$ is 68 in our calculations and it dependents on the convergence accuracy. We also kept 5000 states at each iteration of diagonalization. After that, the Hamiltonian can be solved numerically.

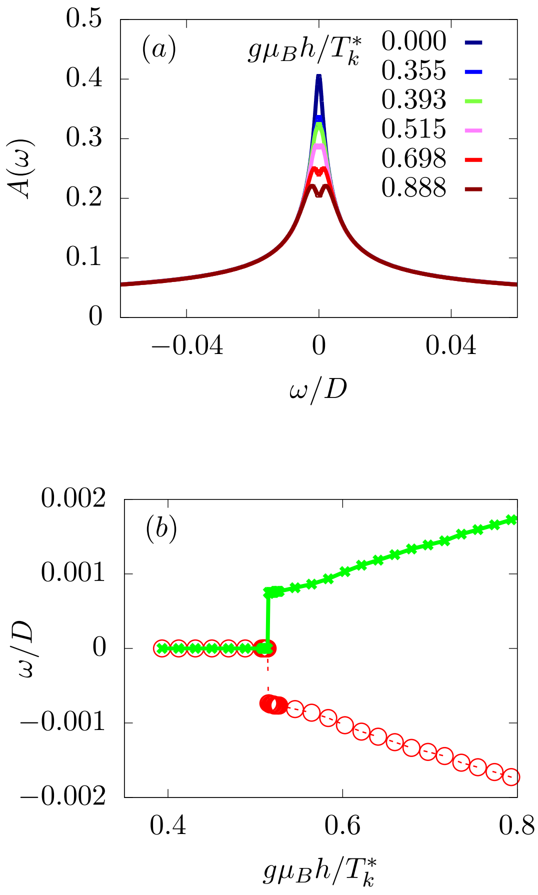


FIG. S2. (Color online) Spectral functions with the magnetic field at $\Delta(T)=0$, $T=0$. a) Kondo resonance and its splitting in the presence of a magnetic field $h$ and b) the positions of the splitting peaks as a function of $h$.

The $T$-matrix is defined as[3]

$$T_\sigma = -i\theta(t)\left\langle \left[O_\sigma(t), O_\sigma(0)^\dagger\right]_+ \right\rangle, \quad O_\sigma = [H_{imp}, f_{0,\sigma}]_+ . \tag{S3}$$

which describes the scattering of conduction electrons off the impurity. Since we know $H_{imp}$, the operator $O_\sigma$ can be written as

$$O_\sigma = J\boldsymbol{S}\cdot\sum_{\sigma'}\frac{1}{2}\boldsymbol{\tau}_{\sigma\sigma'} f_{0,\sigma'} \tag{S4}$$

The spin spectral function is

$$A_\sigma(\omega) = -\frac{1}{\pi} Im\tilde{T}_\sigma(\omega + i\delta) \tag{S5}$$

We obtain the impurity spectral function by summing the up and down spin spectral function[4],

$$A(\omega) = \sum_\sigma A_\sigma(\omega) \tag{S6}$$

where $\tilde{T}$ is the Fourier transformation of $T$ in $\omega$-space. Then, we apply the Full-Density-Matrix(FDM) NRG method[5] in the actual finite temperature spectral function calculations. After that, we accumulate the raw spectral data and using 1000 bins as well as two different broadening kernels, one inside the gap, and another one outside[6]. To calculate the finite temperature spectral function, we use the FDM method for high accuracy[5,7]. It takes advantage of a complete set of the discarded numerical renormalization group eigenstates. Assuming $|s\rangle_n^X$ is the eigenstate of the Wilson chain Hamiltonian at the iteration diagonalization step $n$, $X$ indicates the $K$(kept states) or $D$(discarded states), and the length of the total chain is $N$. Then, we can build the approximate eigenstates of the total Hamiltonian[5] ,

$$H_N|se\rangle_n^X \approx E_s^n|se\rangle_n^X \tag{S7}$$

where $|se\rangle_n^X = |s\rangle_n^X \otimes |e_n\rangle$, and $|e_n\rangle = |\sigma_N\rangle\otimes\cdots\otimes|\sigma_{n+1}\rangle$ is the so-called environmental states and $|\sigma_n\rangle$ is the single site states $|0\rangle$, $|\uparrow\rangle$, $|\downarrow\rangle$ or $|\uparrow\downarrow\rangle$. The $E_s^n$ state has $d^{N-n}$-fold degeneracy. These discarded states from all the iteration diagonalization step can be combined to a complete eigenstates $|se\rangle_n^D$of $H_N$,

$$\sum_{n>n_0}^{N}\sum_{se}|se\rangle_n^D {}_n^D\langle se| = 1 \tag{S8}$$

where $n_0$ is the last step that can be calculated without truncation in the iteration diagonalization. These states are called the 'Anders-Schiller basis'[8,9]. The full density matrix is,

$$\rho \approx \sum_{n>n_0}\sum_{se}|se\rangle_n^D \frac{e^{-\beta E_s^n}}{Z} {}_n^D\langle se| = \sum_{n>n_0}\omega_n\rho_{DD}^n \tag{S9}$$

$\rho_{DD}^n = |se\rangle_n^D {}_n^D\langle se|$ is the density matrix for the *discarded* states at $n$-th($n > n_0$) step of the Wilson chain iteration diagonalization and $\omega_n = d^{N-n}Z_n^D/Z$, where $Z_n^D = \sum_s^D e^{-\beta E_s^n}$, $Z = \sum_{se} e^{-\beta E_s^n}$. Therefore, we always have the following relations,

$$Tr\left[\rho_{DD}^n\right] = 1, \tag{S10}$$

$$\sum_{n>n_0}\omega_n = 1. \tag{S11}$$

The thermal averaged spectral functions becomes,

$$A(\omega) = \sum_{n>n_0}\omega_n A_n(\omega) \tag{S12}$$

$A_n(\omega)$ is the spectral function calculated in the 'Anders-Schiller basis' at $n$-th step of the iteration diagonalization process.

To calculate the finite-$T$ spectral function, we use two different broadening kernels as we mentioned in the main text. Modified log-Gaussian broadening kernel was used in the gap region, and the broadening parameter $\alpha$ is 0.0004. Gaussian broadening kernel was used outside the region and the broadening parameter $\omega_0 = T$. We do

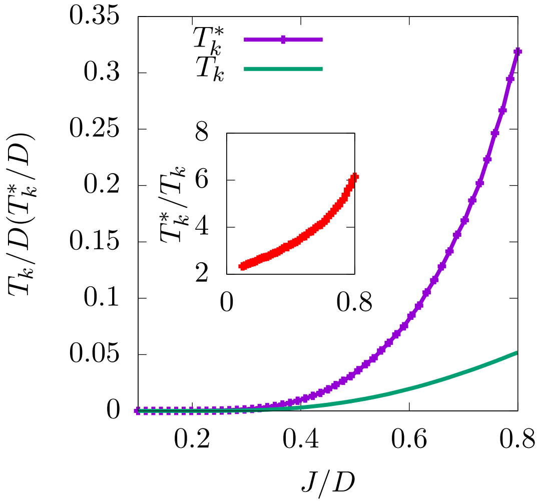


FIG. S3. (Color online). The comparison between $T_k$ and $T_k^*$ as functions of $J/D$. The inset shows the ratio $T_k^*/T_k$ as a function of $J/D$.

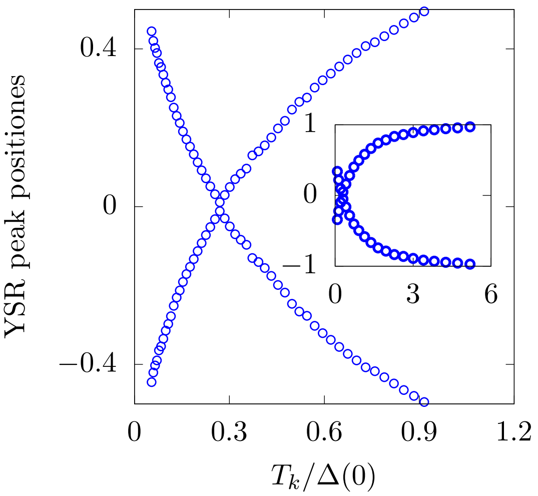


FIG. S4. (Color online) Zero temperature YSR peak positions. The positions of the YSR peaks in the spectral function plotted against $T_k/\Delta(0)$ at $T = 0$. The crossing point is $J_c/D \approx 0.39$ (or $T_k/\Delta(0) = 0.26$).

this broadening and the spectral function calculations by writing the Perl script to call the NRG Ljubljana library.

Because of the BCS gap parameter $\Delta$ is temperature dependent, we also use $\Delta(T)$ instead of the constant number $\Delta$ in the calculations of the temperature dependent spectrum functions. In fact, it's hard to considering a self-consistent process in the NRG to determine the BCS parameter $\Delta(T)$ in the Hamiltonian. Therefore, we keep $\Delta(0)/D = 0.01$ at $T = 0$ and using a phenomenological expression BCS gap formula to simulating the real situation[10],

$$\Delta(T) \approx \delta_{SC} T_c tanh \left[ \frac{\pi}{\delta_{SC}} \sqrt{a \frac{\delta C}{C_N} \left( \frac{T_c}{T} - 1 \right)} \right] \quad \text{(S13)}$$

where $\delta_{SC} = 1.76, a = 2/3, \delta C/C_N = 1.43$. This is a good approximation for the true case with $T \to 0$ and $T \to T_c$.

To test our numerical method, let us study the Kondo problem at $T = 0$ without the SC (or $\Delta(0) = 0$) in the presence of an applied magnetic field $h$. The spectral function exhibits the well-known Kondo resonant behavior at zero energy for weak magnetic field (see Fig.S2(a)), and the resonance peak will split into two as $h$ becoming more significant than a critical value $h_c$ which can be obtained from $g\mu_B h_c/T_k^* \approx 0.51$, here $g = 2$ is the $g$-factor and $\mu_B$ is the Bohr magneton.

These results are consistent with those of Costi's calculation[4]. Besides, we also calculate the peak positions as a function of the magnetic field $h$, and the transition appears to be the first order as shown in Fig.S2(b). Here the another Kondo temperature $T_k^*$[4] is defined as the half-width at the half-maximum (HWHM) of the Kondo resonance at $T = 0$. The comparison of $T_k^*$ and the traditional Kondo temperature $T_k$ as functions of $J$ is shown in Fig.S3. It is easy to see that their difference grows larger as $J$ increases.

Furthermore, we plot the positions of the YSR peaks as functions of $T_k/\Delta(0)$ in Fig.S4. The double YSR peaks emerge from the SC coherent peaks into the gap region as $T_k$ or $J$ changes from 0 to a finite value (not shown here). As $T_k/\Delta(0)$ increases, the separation between the YSR peaks shrinks and it vanishes at $T_k/\Delta(0) \approx 0.26$. From Fig.S1 in Section A of the SM, it indicates that for $T_k/\Delta(0) < 0.26$ or $J/D < 0.39$, the spin state at the impurity site is a doublet, which implies that the impurity spin is not even partially screened. When $T_k/\Delta(0) > 0.26$, the double YSR peaks show up again in the gap, and the spin state becomes a singlet, and the magnetic impurity changes to be nonmagnetic. Similar result was also obtained by other group[1].

Since the spectral function in NRG is computed by broadening the raw delta-peak binned into narrow intervals and is hence a continuous function that can easily be integrated numerically. As we have mentioned in the main text, we numerically calculated the integrated weight of the YSR peaks as a function of $J/D$ at $T = 0$. The integrated weight of the YSR peak is defined as $W_{YSR} = \int_a^b A(\omega) d\omega$[10], where $a$ and $b$ are points to the left and the right of the YSR peak. It is demonstrated there that as $J/D$ approaches 0 and 1, the integrated weight of the YSR peaks goes to 0. The maximum integrated weight comes around $J/D = 0.5$. For $J = 0$, there is no Kondo impurity, and there are no YRS peaks. For $J/D = 1$, the YSR peaks are at the coherent peaks but with zero integrated weight, and that is the typical

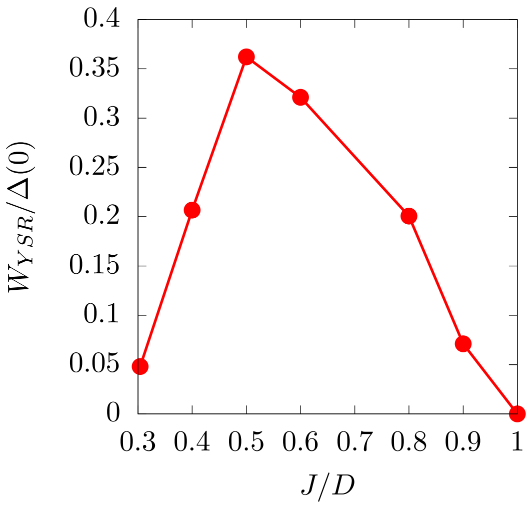


FIG. S5. (Color online) Integrated weight of YSR peak at $T = 0$. The weight goes to zero when YSR peak moves closely to the coherent peak.

characteristics of a nonmagnetic impurity in which the impurity spin paired strongly with the spin of a conduction electron at the impurity site to form a rigid singlet state.

## III. C. THE SQUARE OF THE IMPURITY MAGNETIC MOMENT.

Although the particle number is not conserved in origin Hamiltonian, the system still has spin $U(1)$ symmetry. Thus, the Wilson Chain can be diagonalized in the $S_z$ subspace. After completing the diagonalization process, it is easy to obtain the lowest two energy levels by comparing all the lowest energy values in all of the subspace.

Since the total $S_z$ is a good quantum number, the square of impurity magnetic moment is expressed as[11–13],

$$\langle (S^z_{imp})^2 \rangle = \langle (s^z_{imp} + S^z)^2 \rangle - \langle (S^z)^2 \rangle_0 \qquad \text{(S14)}$$

where $S^z = \sum_{i=1}^{Ns} s^z_i$ and $s^z_i$ is the spin of the Wilson Chain at site $i$. $s^z_{imp}$ is the spin at impurity site. $\langle ... \rangle$ indicates the value is measured in the system with a Kondo impurity while $\langle ... \rangle_0$ represents this measurement for the clean system. Such a quantity reflects the changes in magnetic moment due to the presence of the impurity. If there is no conduction electrons, $\langle (S^z_{imp})^2 \rangle$ is just 0.25. Similarly, it is 0 if there exists no impurity. Thus, Eq.S14 describes the impurity contribution to the square of the magnetic moment. Also, we using the $z - averaging$ and finite temperature NRG algorithm to perform the $T$-dependent thermal properties calculations.

There exist two competing interactions in the system, one is the Kondo coupling, and the other is SC pairing. At the weak Kondo coupling case, all the conduction electrons form Cooper pairs, and the impurity is not able to capture an electron from the Cooper pair. In this case, $\langle (S^z_{imp})^2 \rangle$ is 0.25 or its square root measuring $< S^z_{imp} >$ is 0.5. On the other hand, once the Kondo coupling $J$ becomes stronger but not too much strong such that $T_k/\Delta(0) > 0.26$, the impurity can pair loosely with an electron from a Cooper pair to form a singlet state. However, this electron can go to the sites away from the impurity and still forming a Cooper pair with another electron. Therefore, the impurity may still maintain some of its magnetic behavior. For $J >> J_c$, the impurity can capture an electron, and it may behave like a nonmagnetic impurity as we mentioned in the main text. Moreover, $\langle (S^z_{imp})^2 \rangle$ is 0 if $T_k/\Delta(0) > 0.26$.


* yanchen99@fudan.edu.cn
† ting@uh.edu



1. O. Sakai, Y. Shimizu, H. Shiba, and K. Satori, J. Phys. Soc. Jpn. **62**, 3181 (1993).
2. K. Satori, H. Shiba, O. Sakai, and Y. Shimizu, J. Phys. Soc. Jpn. **61**, 3239 (1992).
3. L. Fritz, S. Florens, and M. Vojta, Phys. Rev. B **74**, 144410 (2006).
4. T. A. Costi, Phys. Rev. Lett. **85**, 1504 (2000).
5. A. Weichselbaum and J. von Delft, Phys. Rev. Lett. **99**, 076402 (2007).
6. T. Hecht, A. Weichselbaum, J. von Delft, and R. Bulla, J. Phys. Condens. Matter **20**, 275213 (2008).
7. L. Merker, A. Weichselbaum, and T. A. Costi, Phys. Rev. B **86**, 075153 (2012).
8. F. B. Anders and A. Schiller, Phys. Rev. Lett. **95**, 196801 (2005).
9. F. B. Anders and A. Schiller, Phys. Rev. B **74**, 245113 (2006).
10. R. Žitko, Phys. Rev. B **93**, 195125 (2016).
11. K. G. Wilson, Rev. Mod. Phys. **47**, 773 (1975).
12. H. R. Krishna-murthy, J. W. Wilkins, and K. G. Wilson, Phys. Rev. B **21**, 1044 (1980).
13. P. S. Cornaglia and C. A. Balseiro, Phys. Rev. B **66**, 115303 (2002).
